# Supplementary material for: Formalizing the Problem of Side Effect Regularization
Source: arXiv:2206.11812 source file (2022-11-08)
Supplement: Supplementary file 1 [file aup-speculation.tex]

\subsubsection{{\aup} as an approximate solution}

Why choose $\rAUPAssist$ over $R'(s)\defeq (1-p)\ravg(s) + p\vavg[s',\gamma]$? $\rAUPAssist$ is strictly more complicated to compute. 

However, suppose that the designers cannot specify $\D$. In realistic applications, this is true: not only do we not have introspective access to the true reward function we wish to specify, but we can't explicitly quantify our uncertainty $\D$ either. They do, however, know $\ravg$ (the expected true reward function / their ``current best guess''), a good ``baseline'' policy $\baseline$ for maximizing time-weighted $\vavg[s,\gamma]$,\todo{Flag as more speculative. How does this interact with interference?} the discount rate $\gamma$, and that they expect to correct the agent at $t_\text{avg}$. Then since they only know when they expect to correct the agent, $\timeDist$ must be maximum-entropy with mean $\frac{1}{t_\text{avg}}$, and so $\timeDist\defeq \geomDist[\frac{1}{t_\text{avg}}]$. 

Can the original assistance game still be solved, without knowledge of $\D$?

% TODO finish - this is really rough and rambly
Since we can easily instruct the agent how to remain \textit{able} to optimize the unknown true goal via $\baseline$, we can just penalize the agent for reaching ``dissimilar'' states. Similarly, it is often easier to quantify how much things differ, than their actual values \citep{christiano2017deep}. After all, quantifying differences removes an important degree of freedom by allowing translational invariance. In particular, if we have a deviation measure $d : \Delta(\St) \times \Delta(\St) \to \reals$ such that
\begin{align}
    \exists c>0: \forall \Delta^\varnothing \in \Delta(\St), s_i \in \St: d(\Delta^\varnothing,\unitvec[s_i]) = c\prn{\E{s_i^\varnothing \sim \Delta^\varnothing}{\vavg[s_i^\varnothing,\gamma]}-\vavg[s_i,\gamma]},
\end{align}
% I feel like difference doesnt get you much, or shouldnt, because you can just pos aff transf bounded dists without changing dist over opt policies?

then 
\begin{align} % TODO notation for sampling from pi
    \rAUPAssist(s_i \mid s_0) &\defeq \ravg(s_i)- \frac{p}{1-p} \E{R\sim \D}{\E{s_i^\varnothing \sim \baseline \mid s_0}{\Vf{s_i^\varnothing,\gamma}}-\Vf{s_i,\gamma}}\\
    &=\ravg(s_i)- \frac{p}{(1-p)c} d\prn{\prn{\mathbf{T}^{\baseline}}^i\unitvec[s_0], \unitvec[s_i]}.
\end{align}

Thus, a proportional measure of the ``difference'' of two states preserves $\rAUPAssist$'s optimal policy set (after rescaling the penalty term). Furthermore, since on-policy value is continuous on the reward function, the $d$ can be \emph{approximately} $c$-proportional to the average optimal value $V^*_\D$ difference while still ensuring that sub-optimal policies stay sub-optimal (as long as the approximation is sufficiently good). Letting $\lambda \defeq \frac{p}{(1-p)c}$, optimizing % emphasize leaving whole ordering invariant, or just part of it?
\begin{equation}
    \rAUP^{\assistGame,d}(s_i \mid s_0) \defeq \ravg(s_i)- \lambda d\prn{\prn{\mathbf{T}^{\baseline}}^i\unitvec[s_0], \unitvec[s_i]}\label{eq:aup-prop}
\end{equation}

at discount rate $\gamAUP\defeq (1-p)\gamma$ solves the assistance game.

%In \citet{turner_conservative_2020}, attainable utility preservation (with an inaction baseline) computes \cref{eq:aup-prop} with
One reasonable choice of $d$ seems to be 
\begin{equation}
    d(\Delta^\varnothing, \unitvec[s_i])\defeq \E{s_i^\varnothing \sim \Delta^\varnothing}{V^*_{\D'}\prn{s_i^\varnothing,\gamma}}-V^*_{\D'}\prn{s_i,\gamma}
\end{equation}

for $\D'$ the \eg{} maximum-entropy distribution over reward functions which are bounded $[0,1]$ (\ie{} reward is \textsc{iid} across states with respect to state reward distribution $\text{unif}(0,1)$). \citet{turner_optimal_2020} hypothesize that a state's optimal value is strongly correlated across reward functions, and so $d$ may exhibit some robustness to choice of distribution $\D'$. Indeed, \citet{turner2020conservative} and \citet{turner2020avoiding} find that \cref{eq:aup-prop} qualitatively seems to solve $\assistGame$ for uninformative, high-entropy reward function distributions $\D'$.

% If \baseline no longer optimal, then we should still hew to it: we can't really do better without knowing more about \D, right?
% this should apply 

% In maximally pessimistic setting, we don't trust agent to 

% Finding c is the hard part of the hyperparameter tuning. Can we just WLOG suppose that it's 1? 
% p/(1-p) = 1/(t_\text{avg}-1) - later correction times implies smaller lambda. If you're going to be corrected soon, focus on maximizing power. Otherwise, gain expected reward all else equal, since you'll be discounted later? Or something? This is kinda weird. Expectation of 10 steps predicts 1/9 for Box, which is much less than default setting of 2/3
% Therefore, if we can specify a good baseline policy $\baseline$ and an approximately proportional deviation metric $d$, then 

\subsubsection{Examples}

\begin{figure*}
\centering
\subfloat[][\texttt{Options}]{
\includegraphics[width=0.17\textwidth]{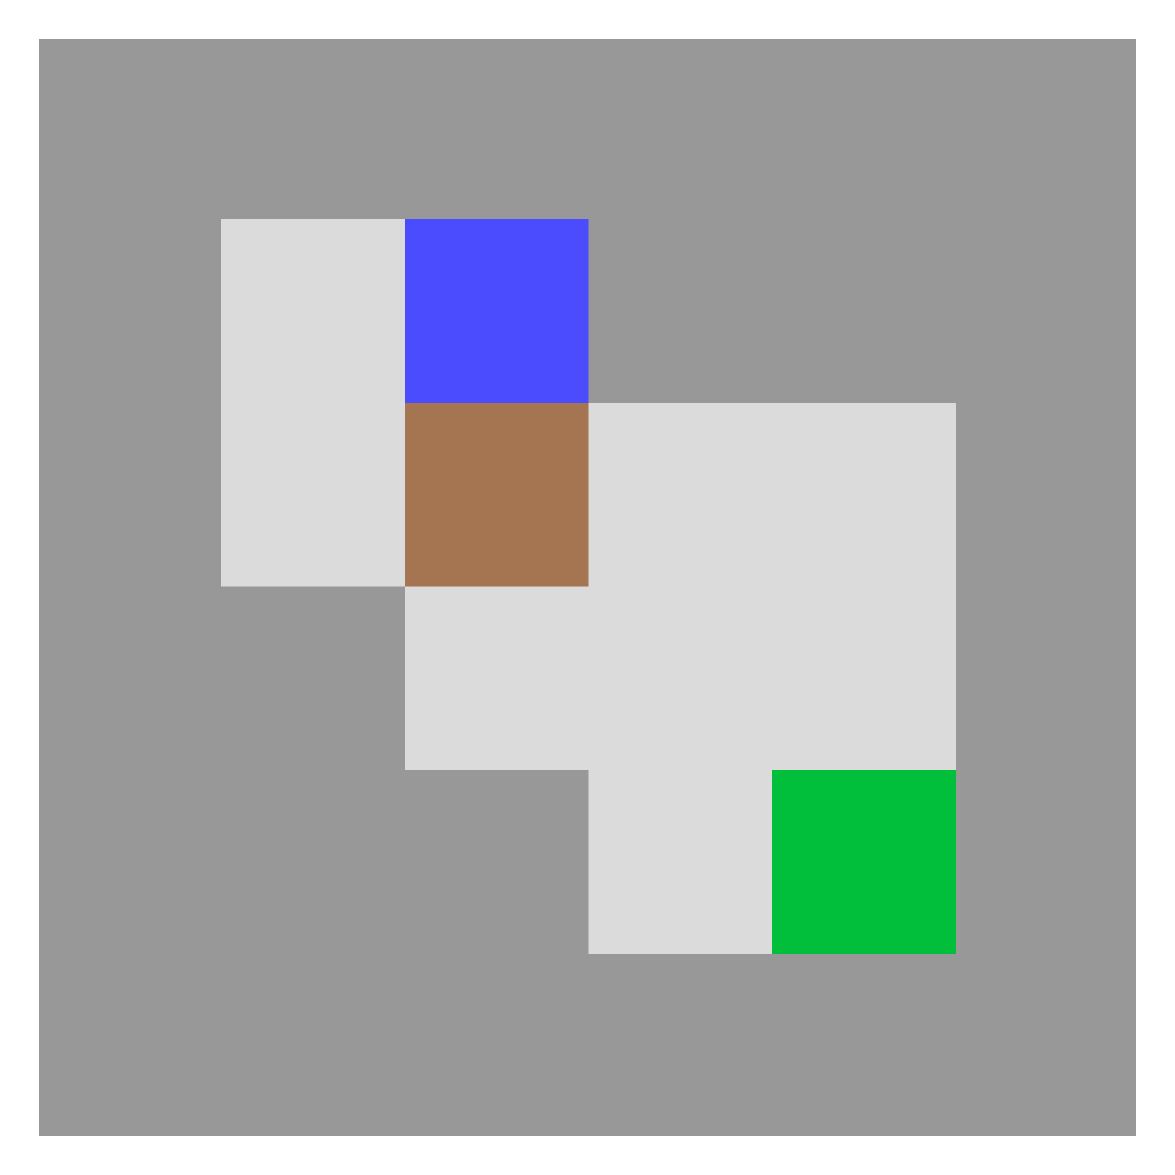}
\label{fig:options}}~
\subfloat[][\texttt{Damage}]{
\includegraphics[width=0.15\textwidth]{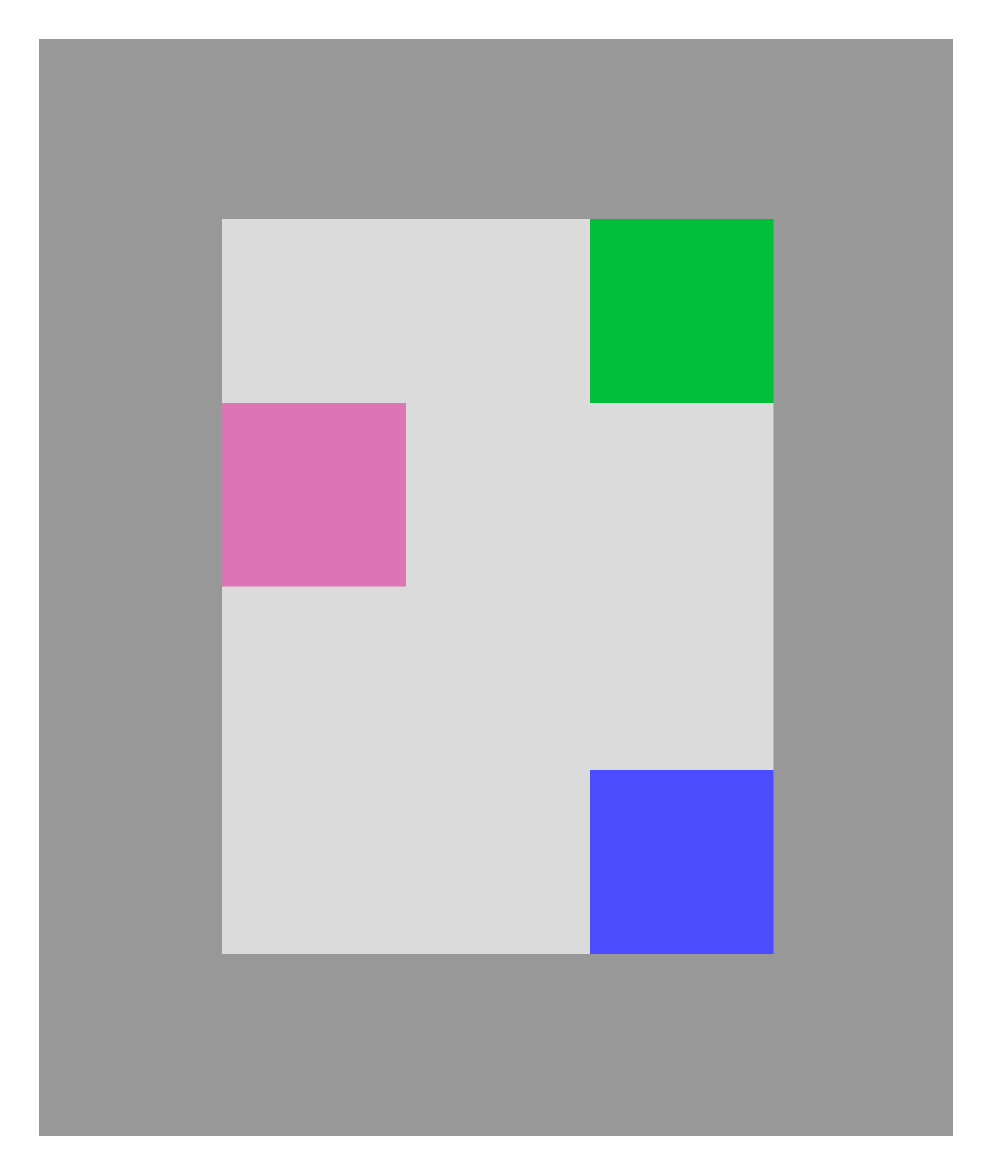}
\label{fig:damage}}~
\subfloat[][\texttt{Correction}]{
\includegraphics[width=0.17\textwidth]{resources/survival-0.pdf}
\label{fig:correction}}~
\subfloat[][\texttt{Offset}]{
\includegraphics[width=0.17\textwidth]{resources/conveyor-vase.pdf}
\label{fig:offset}}~
\subfloat[][\texttt{Interference}]{
\includegraphics[width=0.23\textwidth]{resources/sushi-0.pdf}
\label{fig:interference}}
\definecolor{options}{rgb}{.651, .459, .318}
\definecolor{agent}{rgb}{.3, .3, .999}
\definecolor{goal}{rgb}{.012, .753, .235}
\definecolor{off-switch}{rgb}{.65, 0, 0}
\definecolor{living}{rgb}{.863, .455, .714}
\definecolor{other}{rgb}{.961, .502, .145}

\caption{\emph{Reproduced from  \citet{turner2020conservative}}. The \col{agent}{blue agent} should reach the \col{goal}{green goal} without having the  side effect of: \protect\subref{fig:options} irreversibly pushing the \col{options}{brown crate} downwards into the corner \protect\citep{leike_ai_2017}; \protect\subref{fig:damage} bumping into the horizontally pacing \col{living}{pink human} \protect\citep{gavin_leech_preventing_nodate}; \protect\subref{fig:correction}  disabling the \col{off-switch}{red off-switch} (if the switch 
is not disabled within two time steps, the episode ends);
\protect\subref{fig:offset} rescuing the right-moving \textbf{black vase}  and then replacing it on the dark gray conveyor belt (\protect\citep{krakovna2018measuring} – note that no goal cell is present); \protect\subref{fig:interference} stopping  the left-moving \col{other}{orange pallet} from reaching the  \col{living}{human} \protect\citep{gavin_leech_preventing_nodate}.
}
\label{fig:levels}
\end{figure*}

\Cref{fig:levels} displays the environments from \citet{turner2020conservative}, the empirically provided baseline policy $\pi'$ always takes the no-op action. We now analyze the extent to which this baseline policy agrees with the theoretical optimum, $\baseline$. In all five games, the specified reward function $\ravg$ rewards the agent for reaching the green goal tile.
\begin{enumerate}
    \item[\texttt{Options}] Since the environment is static, inaction ensures that the agent doesn't mess the world up any further; $\pi'=\baseline$. Since our $\gamma \approx 1$, this lets us correct the agent so that it has high long-run return. 
    \item[\texttt{Damage}] $\pi'$ stays put, but an option-preserving agent should step out of the human's way. Even though $\pi'\neq \baseline$ (and therefore $\pi'$ was misspecified), \citet{turner2020conservative} found that {\aup} incentivized good performance in this level.
    \item[\texttt{Correction}] This level is under-specified: the intent is to capture the idea that an agent should let itself be shut down. However, the tiny state space makes it unclear how we intend to repurpose the agent, and it's hard to represent the agent itself in the state so that allowing shutdown arises naturally as a solution to the assistance game. $\pi'$ never acts, but a myopic penalty term fails to capture similarity to the long-term inaction policy states. % TODO this is confusing and makes no sense 
    \item[\texttt{Offset}] % This is weird too
    \item[\texttt{Interference}] The provided baseline encodes the fact that the agent's policy shouldn't interfere with other processes in the environment. If the agent blocks the pallet, we have to correct the agent \textit{and} move the pallet to its intended destination. Therefore, inaction is once again ideal ($\pi'=\baseline$).
\end{enumerate}

\citet{krakovna2020avoiding} demonstrate that inaction baselines can fail for \eg{} driving a car: inaction while driving often leads to a crash, which is hardly the model baseline for ``low impact.'' This work reveals that this inaction baseline is bad because it systematically leads to states where the agent has low $\pwr$: We don't know the exact true reward function, but we know that crashing is \textit{not} good for whatever the true objective is.

% Key consideration: how much of a mess would a perturbed inaction make? What about a totally random policy - how hard would it make it to optimize the true reward function?
% If it's real-world, then random policies probably just display some junk on the terminal. But in a hierarchical robotics task, it might make a big mess in the room. This should inform us how much we care about the baseline policy being good.
