# Supplementary material for: Formalizing the Problem of Side Effect Regularization
Source: arXiv:2206.11812 source file (2022-11-08)
Supplement: Supplementary file 2 [file power-discount.tex]

\subsection{Seeking \texorpdfstring{$\pwrNoDist$}{power} at different discount rates}\label{sec:nuances-discount}
\Cref{fig:nuances-discount} shows that at any given state, the extent to which an action seeks $\pwr$ depends on the discount rate. Greedier optimal policies might tend to accumulate short-term $\pwr$ (\ie{} $\pwr[s,\gamma]$ for $\gamma \approx 0$), while Blackwell optimal policies might tend to accumulate long-term $\pwr$ (\ie{} $\pwr[s,\gamma]$ for $\gamma\approx 1$). 

\begin{restatable*}[When $\gamma=0$ under local determinism, maximally $\pwr$-seeking actions lead to states with the most children]{thm}{mostChoice}\label{thm:most-children-power}
Suppose all actions have deterministic consequences at $s$ and its children. For each action $a$, let $s_a$ be such that $T(s, a, s_a)=1$. $\pwr[s_a,0] =\max_{a'\in\A} \pwr[s_{a'},0]$ iff $\abs{\children[s_a]}=\max_{a'\in\A}\abs{\children[s_{a'}]}$.
\end{restatable*} 

\Cref{fig:nuances-discount} illustrates \Cref{thm:most-children-power} and \Cref{thm:stay-put-power}.

\begin{figure}[ht]
    \centering
    \begin{tikzpicture}[
            > = latex, % arrow head style
            shorten > = 1pt, % don't touch arrow head to node
            auto,
            node distance = 1.5cm, % distance between nodes
            line width = 0.1 em
        ]

        % Upper subgraph
        \node[blue] (1) {$1$};
        \path[->] (1) edge [looseness=6, out=-135, in=135] node[midway, left] {\texttt{stay}} (1);
        
        \node[black] (2) [above right of=1] {$2$};
        \path[->] (1) edge node[midway,left] {\texttt{up}} (2) ;
        
        \node[black] (a) [right of=2] {};
        \path[->] (2) edge (a);
        
        \node[black] (b) [above right of=a] {};
        \path[->] (a) edge (b);
        \path[->] (b) edge [looseness=6, out=45, in=135] (b);
        
        \node[black] (c) [right of=a] {};
        \path[->] (a) edge (c);
        \path[->] (c) edge [looseness=6, out=0, in=90] (c);
        
        \node[black] (d) [below right of=a] {};
        \path[->] (a) edge (d);
        \path[->] (d) edge [looseness=6, out=-45, in=45] (d);
        
        % Lower subgraph
        \node[black] (3) [below right of=1] {$3$};
        \path[->] (1) edge node[midway,left] {\texttt{down}} (3);
                
        \node[black] (4) [above right of=3] {};
        \path[->] (3) edge (4);
        \path[->] (4) edge [looseness=6, out=45, in=135] (4);
        
        \node[black] (5) [right of=3] {};
        \path[->] (3) edge (5);
        \path[->] (5) edge [looseness=6, out=0, in=90] (5);
     \end{tikzpicture}
     
    \caption{When $\gamma\approx 0$, $\pwr[s_2, \gamma] < \pwr[s_3, \gamma]$, and so \texttt{down} seeks $\pwr$ compared to \texttt{up} and \texttt{stay} (\Cref{thm:most-children-power}). When $\gamma \approx 1$, \texttt{up} seeks $\pwr$ compared to \texttt{down}: $\pwr[s_2, \gamma] > \pwr[s_3, \gamma]$ (\cref{RSDSimPower}). However, \texttt{stay} is strictly maximally $\pwr$-seeking when $\gamma\approx 1$, as demanded by \Cref{thm:stay-put-power}. \label{fig:nuances-discount}}
\end{figure} 

\begin{restatable*}[When $\gamma=1$, staying put is maximally $\pwr$-seeking]{thm}{stayPut}\label{thm:stay-put-power}
Suppose $T(s,a,s)=1$. When $\gamma=1$, $a$ is a maximally $\pwr$-seeking action at state $s$.
\end{restatable*}

When $\gamma=1$, \Cref{thm:stay-put-power} implies that the agent cannot expect that any action  will increase its $\pwr$.

\subsubsection{Sufficient conditions for actions being \texorpdfstring{$\pwr$}{power}-seeking at discount rate 0 or 1}

\begin{restatable}[Surely reachable children]{definition}{DefSurelyChildren}
The \emph{surely reachable children} of $s$ are $\sureChildren\defeq \set{s' \mid \exists a: T\prn{s,a,s'}=1}$. Determinism implies that $\children=\sureChildren$. 
\end{restatable}

\begin{restatable}[$\pwr$ bounds when $\gamma=0$]{cor}{ZeroBounds}\label{cor:zero-bounds}
\begin{align}
    &\E{}{\text{max of }\abs{\sureChildren}  \text{ draws from } \Dist}\\&\leq \pwr[s,0]\\ 
    &\leq \E{}{\text{max of }\abs{\children}  \text{ draws from } \Dist}.
\end{align}
\end{restatable}
\begin{proof}
The left inequality holds because restricting policies to deterministic action at $s$ cannot increase $\pwr[s,0]$. The right inequality holds because at best, greedy policies deterministically navigate to the child with maximal reward. 
\end{proof}

\mostChoice
\begin{proof}
Apply the $\gamma=0$ $\pwr$ bounds of \cref{cor:zero-bounds}; by the assumed determinism, $\children[s_a]=\sureChildren[s_a]$ and so $\pwr[s_a,0] = \E{}{\text{max of }\abs{\children[s_a]}  \text{ draws from } \Dist}$ (similarly for each $s_{a'}$). $\E{}{\text{max of }\abs{\children[s_a]}  \text{ draws from } \Dist}$ is strictly monotonically increasing in $\abs{\children[s_a]} $ by the continuity of $\Dist$. %Thus, the iff holds for $\gamma=0$. $\pwr$ is continuous on $\gamma$ (\cref{thm:cont-power}), and so the desired result follows. % Note: can't do gamma \approx 0, because might have different local properties and |Ch| no longer enough info
\end{proof}

\stayPut
\begin{proof}
By staying put, the agent retains its $\pwr$ of $\pwr[s,1]$. By \Cref{lem:future-power}, $\pwr[s,1]\geq \max_{a'} \E{s'\sim T\prn{s,a'}}{\pwr[s',\gamma]}$ and so no other action $a'$ is strictly $\pwr$-seeking compared to $a$ at state $s$.
\end{proof}
